# Supplementary material for: Mitigating Configuration Differences Between Development and Production Environments: A Catalog of Strategies
Source: arXiv:2505.09392 source file (2025-05-15)
Supplement: Supplementary file 1 [file Semi-structuredQuestionnaire.pdf]

**Dados demográficos**

1. Qual sua idade?
2. Qual sua profissão?
3. Fale-me sobre a sua empresa, a sua função dentro da empresa e o projeto em que trabalha atualmente.
    a. Há quanto tempo você está neste cargo?

**Perguntas relacionadas ao ambiente de desenvolvimento**

1. O ambiente de desenvolvimento **é dentro da empresa, na máquina do desenvolvedor, na nuvem ou híbrido**?
    a. Por que vocês optaram por essa forma?
2. Esse seu ambiente de desenvolvimento é criado para cada projeto ou existe um geral para todos os projetos?
    a. Por que vocês optaram por essa forma?
    b. Como é feita a construção desse ambiente de desenvolvimento?
3. Existe durante o processo de construção de ambiente de desenvolvimento alguma rotina voltada para a **automatização**?
    a. Em caso positivo, porque vocês **estão** automatizando o ambiente de desenvolvimento?

    b. Quais **tipos** de rotinas foram automatizadas?

    c. Vocês têm ou tiveram alguma **dificuldade** para automatizar essas rotinas?

    d. Vocês percebem algum tipo de **benefício** que surgiu ao automatizar essas rotinas?

    e. Vocês **testam** essas rotinas de build de ambiente?

        i. **Como** vocês **testam** essas rotinas?

        ii. Vocês têm **dificuldades** em testar? Se sim, quais?

4. Você pode nos contar como é feita a **build** do produto no ambiente de desenvolvimento?
    a. Vocês usam **continuous integration**?

        i. Quais as **práticas** de continuous integration vocês usam?

        ii. Como vocês **implementaram** essas práticas?

        iii. Quais **dificuldades** vocês tiveram durante a fase de implantação do continuous integration?

5. Vocês têm algum tipo de f**erramenta de automação** para **simular** uma recuperação de **falhas** na produção?
    a. Quais **ferramentas** vocês escolheram?

**Perguntas relacionadas ao ambiente de Produção**

6. Você tem acesso ao ambiente de produção?
    a. Como é escolhido quem será o responsável do Time por implantar a solução na produção?
7. Esse ambiente de produção **é dentro da empresa, na nuvem ou híbrido**?
    a. Por que vocês optaram por essa forma?
8. Esse seu ambiente de produção é criado para cada projeto ou existe um geral para todos os projetos?
    a. Por que vocês optaram por essa forma?
9. Como é feita a construção desse ambiente de produção?
    a. Durante o processo de construção de ambiente, existe alguma rotina que seja **automatizada?**
    b. Por que vocês optaram por **automatizar** o ambiente de produção?
    c. Quais **tipos** de rotinas foram automatizadas?
    d. Qual delas foi mais **priorizada** e o porquê?
    e. Vocês têm ou tiveram alguma **dificuldade** para automatizar essas rotinas?
    f. Vocês percebem algum tipo de **benefício** que surgiu dessa frente de automatizar essas rotinas?
10. Você pode nos contar como é feito o **deploy**?
    a. Quanto tempo leva em **média** para uma **mudança** percorrer do commit até a produção?
    b. Vocês usam **continuous delivery**?
        i. Quais as **práticas** de continuous delivery vocês usam?
        ii. Como vocês **implementaram** essas práticas?
        iii. Quais **dificuldades** vocês tiveram durante a fase de implantação do continuous delivery?
11. Vocês têm algum tipo de **ferramenta de automação** para se recuperar de **falhas** na produção?
    a. Por que vocês optaram por essas **ferramentas**?

**Ambientes separados**

12. Como vocês **mitigam** as diferenças de configuração, segurança, serviços e conectividade entre os ambientes?
    a. Alguma rotina deste processo que visa **mitigar** as diferenças entre os ambientes é **automatizada**?
    b. Quais ferramentas?
13. Essas ações de mitigação são **suficientes**?
    a. Por quê?

Entrevistas + Rapid Review

Proposta de um Guia (Guide Line ou CookBook)

Validar o Guia

RQ - Como as empresas **constroem** os seus ambientes de desenvolvimento e produção?

RQ - Quais as ações que são tomadas pelo time para **mitigar** as diferenças entre os ambientes?

RQ - São **suficientes** essas ações do time para **mitigar** as diferenças entre os ambientes?

RQ - Quais os **benefícios** percebidos através da automatização nos ambientes de desenvolvimento e produção.

RQ - Quais as **dificuldades** percebidas no processo da automatização nos ambientes de desenvolvimento e produção.
